# Supplementary material for: Experimental Scattershot Boson Sampling
Source: arXiv:1505.03708 ancillary file (2015-05-14)
Supplement: Supplementary file 1 [file SupplementaryMaterials.pdf]

# Experimental Scattershot Boson Sampling - Supplementary Materials

Marco Bentivegna,<sup>1</sup> Nicolò Spagnolo,<sup>1</sup> Chiara Vitelli,<sup>1,2</sup> Fulvio Flamini,<sup>1</sup>  
Niko Viggianiello,<sup>1</sup> Ludovico Latmiral,<sup>1</sup> Paolo Mataloni,<sup>1</sup> Daniel J. Brod,<sup>3</sup>  
Ernesto F. Galvão,<sup>4</sup> Andrea Crespi,<sup>5,6</sup> Roberta Ramponi,<sup>5,6</sup> Roberto Osellame,<sup>5,6</sup>  
Fabio Sciarrino<sup>1\*</sup>

<sup>1</sup>Dipartimento di Fisica, Sapienza Università di Roma,  
Piazzale Aldo Moro 5, I-00185 Roma, Italy

<sup>2</sup>Center of Life NanoScience @ La Sapienza, Istituto Italiano di Tecnologia,  
Viale Regina Elena, 255, I-00185 Roma, Italy

<sup>3</sup>Perimeter Institute for Theoretical Physics,  
31 Caroline Street North, Waterloo, ON N2L 2Y5, Canada

<sup>4</sup> Instituto de Física, Universidade Federal Fluminense,  
Av. Gal. Milton Tavares de Souza s/n, Niterói, RJ, 24210-340, Brazil

<sup>5</sup>Istituto di Fotonica e Nanotecnologie, Consiglio Nazionale delle Ricerche (IFN-CNR),  
Piazza Leonardo da Vinci, 32, I-20133 Milano, Italy

<sup>6</sup>Dipartimento di Fisica, Politecnico di Milano,  
Piazza Leonardo da Vinci, 32, I-20133 Milano, Italy

\* E-mail: fabio.sciarrino@uniroma1.it

## Experimental details

Single photons were generated in six equal parametric down conversion (PDC) sources, occurring in three separated 2 mm thick nonlinear crystals (BBO) injected by a 680 mW pulsed pump field ( $\lambda = 392.5$  nm). The generated 2-photon pairs were centered at 785 nm and filtered by 3 nm interferential filters (Semrock, rectangular shaped). The different generation efficiencies of the three crystals were due to different focalization conditions and impinging pump power.

Typical count rates of singles and coincidences for the three crystals were, respectively: 200kHz and 35kHz for the first one; 130kHz and 20kHz for the second one; 70 kHz and 14 kHz for the third one.

The 3-photon input state for the 9-mode chip was obtained by PDC generation from the first crystal, with one of the four emitted photons used as a trigger. The other three photons, properly synchronized, were coupled into polarization compensated single-mode fibers, and then injected into the chip. In the case of the 9-mode chip experiment, the input states were changed manually by connecting a fiber array to 20 different sets of input modes of the chip.

The 13-mode chip was then used to implement the complete scattershot version of the Boson Sampling experiment, with the three crystals reproducing six PDC sources. The first one belonging to the first crystal was adopted to inject two fixed input modes of the chip (number 6 and number 8), while another photon was injected shot by shot coming from one of the five remaining PDC sources. The third heralded photon coming from the first crystal and the other four heralded photons from the second and third crystals were connected to eight different input modes of the chip, after passing through a polarization compensation stage and independent delay lines. The injected modes of the chip were number 7 from the first crystal, number 9 and number 11 from the second crystal and number 13 and a cyclically varied number 1,2,3,12 via a fiber switcher from the third crystal. The final detection rate for 3-photon events after the propagation through the chip was  $\sim 30$  coincidences per hour, with an overall efficiency deriving from the coupling efficiency from the source to the input fiber array ( $\sim 0.3$ ), the coupling between the fiber array and the chip ( $\sim 0.6$ ), the transmission efficiency of the chip ( $\sim 0.25$ ) and the coupling between the chip and the multimode output fiber array ( $\sim 0.85$ ).

We then evaluated the enhancement in the event rate related to the Scattershot approach in the 13-mode chip with respect to the standard fixed-input Boson Sampling in the 9-mode chip. By comparing the coincidence rates in the two cases and considering the different transmission efficiencies of the two devices, we observed an enhancement in the measured event rate of a factor  $\sim 3.4$ . This is consistent with the raw estimate based on source coincidence rates, *i.e.*  $R = (35kHz + 2 \times 20kHz + 2 \times 14kHz)/35kHz \sim 3$ . We observe that the 9-mode fixed input

experiment was performed with the sources of the first crystal, which presents higher generation rate due to an optimized optical configuration. By comparing the Scattershot approach with a source of average brilliance, the enhancement increases up to a factor 4.5.

At the output of both 9- and 13-mode chips, multimode fibers were connected to single photon counting detectors and an electronic data acquisition system allowed to register events with an arbitrary number of photons. A timing circuit driven by the five trigger signals controlled both the conditioning input circuit and the four-fold coincidences discrimination and detection circuit. The circuit generates the handshake signal sent to the National PCI-6503 board used for recognising the pattern. We then analyzed data corresponding to 2- and 3-photon interference inside the chip, i.e. fourfold coincidences belonging either to the 1 trigger-3 injected photons events or to the 2 trigger-2 injected photons ones. We recorded events corresponding to all possible 3-mode inputs for 3-photon events. In the case of 2-photon events, because of limitations in the electronic acquisition systems, we could record only events corresponding to two specific 2-mode input combinations. This was imposed by the limited number of bits available to record the output events with the adopted electronic board.

An average estimation of the photon indistinguishability is 0.65-0.75 depending on the photon polarization for photons generated by different sources and 0.95 for photons belonging to the same pair. These estimations are performed by measuring the visibility of Hong-Ou-Mandel ( $I$ ) interference in a symmetric 50/50 beam-splitter, as shown in Fig. 1.

## Synchronization between single photons inside the chip

The key point for the correct functioning of the scattershot experiment relies on the exact synchronization of the arrival time of single photons inside the chip. Temporal matching inside the chip was achieved by exploiting 2-photon Hong-Ou-Mandel interference for paths travelled by photons belonging to the same pairs. The amplification of an attenuated coherent pulse injected into different crystals was in turn exploited to synchronize photons belonging to independent pairs.

1) *Photons belonging to the same crystal.* Single PDC pairs from a given crystal were generated at a sufficient rate to perform HOM experiments. For a given pair of input modes, Hong-Ou-Mandel dips (and peaks) were recorded by counting output coincidences as a function of the spatial mismatch between the two photons entering the chip, adjusted via delay-lines. This task was performed for every combination of output pairs containing a fixed trigger mode. More specifically, Fig. 2 shows Hong-Ou-Mandel dips (or peaks) corresponding to the following

choices of input and output modes: **a**, input modes (6,7), output modes (9,6); **b**, input modes (5,9), output modes (3,7).

2) *Photons belonging to different crystals.* To temporally match photons generated by different crystals, the amplification of a highly attenuated coherent beam was exploited. The choice of using an optical parametric amplifier based on stimulated emission (2) in the synchronization process is due to the need to overcome the lower rate of independent generation of PDC photon pairs by two different sources. The PDC Hamiltonian of the amplifier reads:

$$\mathcal{H} = i\hbar\chi \left( \hat{a}_s^\dagger \hat{a}_i^\dagger - \hat{a}_s \hat{a}_i \right) \quad (1)$$

where  $\hat{a}_s^\dagger(\hat{a}_i^\dagger)$  is the creation operator for the signal (idler) mode and  $\chi$  is proportional to the amplitude of the pump and to the second-order susceptibility of the crystal. By inputting a coherent beam in the signal mode and the vacuum in the idler one the final state reads:

$$|\psi\rangle = |\alpha\rangle_s |0\rangle_i + g\hat{a}_s^\dagger |\alpha\rangle_s |1\rangle_i \quad (2)$$

where  $g = \chi t \ll 1$ . The synchronization of the coherent beam on the signal mode with the pump beam then produced an amplified field on the idler mode. Such matching procedure was realized onto the three crystals (see Fig. 3) and the idler fields belonging to two different crystals were injected into the chip. The Hong-Ou-Mandel dips (or peaks) observed at the output of the chip are shown in Fig. 4, corresponding to injection of photons coming from: **a** crystal 1 and crystal 2 and **b** crystal 1 and crystal 3.

## Validation of Boson Sampling data

Here we provide more details on the validation of Boson Sampling data. More specifically, we discuss how to evaluate the two main sources of experimental imperfections.

The first imperfection to be addressed is the presence of partial photon distinguishability between the generated photons. In our case, for the 13-modes device the input states correspond to input  $(6, j, 8)$ , where  $j$  varies depending on which of the heralded sources ( $S_1, S_3, S_4, S_5$  and  $S_6$ ) emits a photon pair. Photons I and III, corresponding to the fixed inputs 6 and 8, were generated from the same source and present a high degree of indistinguishability. The heralded photon injected in the third mode  $j$  was emitted from a different source, thus presenting a lower degree of distinguishability. In the validation process we took this effect into account in the calculation of the probabilities  $p_i^{\text{ind}}$  for the Boson Sampling case. The input state can be modeled

by a density matrix of the form  $\rho = p^2|1, 1, 1\rangle\langle 1, 1, 1| + (1-p^2)|1, 0, 1\rangle\langle 1, 0, 1| \otimes |0, 1, 0\rangle\langle 0, 1, 0|$ , being  $p$  the degree of indistinguishability between two photons belonging to different pairs and  $|\alpha, \beta, \gamma\rangle$  the number of photons in input modes  $(6, j, 8)$ . The output probability is then evaluated according to the permanent formula for the density matrix  $\rho$ , and is thus a mixture of a genuine three-photon term plus a contribution with only two-photon interference.

Due to imperfections in the fabrication process, the real unitary implemented by the chip is slightly different from the theoretical one. In the validation process, the necessary probabilities  $p_i^{\text{ind}}$  and  $q_i^{\text{dis}}$  were evaluated from the theoretical expected unitary. Its adoption in the validation tests may then produce a slight deviation from the expected trend. We then performed some numerical simulations to estimate the effect of the difference between the implemented and the expected unitary (see the darker cones in Fig. 4 of the main text). The expected  $1\sigma$  and  $2\sigma$  areas were calculated simulating a large number of unitaries, with parameters randomly fluctuating around theoretical values within fabrication tolerances. Statistical fluctuations of the data around an average line are thus accompanied by a constant shift in the derivative, due to the fixed difference between theoretical and effective unitary. The fact that the areas are always contained in the upper semiplane (for Boson Sampling data) or in the lower semiplane (for Uniform Sampler and Distinguishable Sampler) ensure that the validation procedure is robust against experimental noise in the fabrication process.

## Variation distance between observed and theoretical probabilities

In small-scale Boson Sampling experiments it is possible to reconstruct experimentally the output probability distribution by sampling a sufficient number of events. A comparison with the expected theoretical distribution (based on the chip's fabrication specifications) can be performed by calculating the variation distance  $d = 1/2 \sum_i |p_i^t - p_i^e|$ ,  $p_i^t$  and  $p_i^e$  being, respectively, the theoretical and experimental distributions. When dealing with large-scale experiments, the output distributions can no longer be directly reconstructed due to the large sample size required. In the reported 13-mode Scattershot Boson Sampling experiment, the number of sampled events was 5002, corresponding to an average of only 2.2 events per input-output configuration.

To illustrate the expected effect of fabrication errors and limited sample size in the evaluation of the variation distance between experimental and theoretical distributions, we performed a numerical simulation of our Scattershot experiments with the 13-mode interferometer. Our ensemble of simulated interferometers incorporate errors in the chip parameters that correspond to the expected fabrication tolerances. The results are reported in Fig. 5, where the inputs were

randomly generated according to the experimentally observed input distribution due to the different source rates. There is a complete, different output distribution for each different input used. For the ensemble of chip unitaries incorporating manufacturing errors, we observe that the distance  $d$  saturates after about  $10^4$  events. The experimental value of the variation distance  $d$ , obtained from the 5002 sampled events, is compatible with what is expected from the numerical simulation.

We can also model a situation in which our physical interferometer perfectly matches the theoretical specification. One way to approximate this situation would be to obtain a good classical description of the interferometer via an efficient chip tomography scheme. In this case, as the sample size increases we observe a decrease in the variation distance, as the inferred probabilities converge to their theoretically expected values (in our simulation,  $d < 0.06$  for  $N_{\text{events}} > 5 \times 10^4$ ).

## Noise due to higher-order photon generation effects

The probabilistic nature of parametric down-conversion sources and the limited efficiency of the triggering detectors result in a finite probability that unwanted extra photons are injected in the chip. This contributes to noise in Scattershot Boson Sampling experiments. Let us consider our specific scheme, where two types of such noise contributions may arise. The first one is the effect of higher-order terms (when a single source outputs four photons or more, instead of two, in the same pump pulse): this noise contribution also occurs in the standard Boson Sampling protocol, and has been well characterized in Ref. (3). The second type of contribution is peculiar to the Scattershot Boson Sampling set-up: only the first-order effect happens, but on a larger number of sources than those effectively heralded. In this section we analyze these two contributions to experimental noise, and also discuss how high-speed shutters can be used to prevent the second type of heralding errors in future, larger Scattershot Boson Sampling experiments.

First, let us estimate the relative importance of higher-order contributions in the photon generation process, with our specific experiment in mind. Each source  $S_\alpha$  in Fig. 2 of the main text is described by the interaction Hamiltonian  $\mathcal{H} = i\hbar\chi(a_\pi^\dagger b_{\pi_\perp}^\dagger - a_\pi b_{\pi_\perp})$ , where  $\chi$  is the nonlinear coefficient of the process, and  $\{a_\pi, b_{\pi_\perp}\}$  are the field operators associated with the different output spatial modes and polarization states  $\{\pi, \pi_\perp\}$  of the source. The output state of

each source  $S_\alpha$  is:

$$|\Psi_{S_\alpha}\rangle \sim [I + g(a_\pi^\dagger b_{\pi_\perp}^\dagger) + \frac{g^2}{2!}(a_\pi^\dagger b_{\pi_\perp}^\dagger)^2]|00\rangle = |00\rangle + g|11\rangle + g^2|22\rangle \quad (3)$$

where  $g = \chi t$ . In our experiment, a correctly heralded input state corresponds to the generation of a pair from source  $S_2$ , with both photons injected into the interferometer in modes (6,8), and an extra heralded photon from an additional source  $S_{\alpha \neq 2}$ . This event is successfully heralded and detected with probability  $\eta_D^3 \eta_T g^4$ , where  $\eta_D$  is the overall transmission and detection efficiency and  $\eta_T$  the overall triggering efficiency. In our experiment, the main contributions for the overall efficiency  $\eta_D$  can be divided in injection efficiency ( $\eta_{\text{inj}} \sim 0.15$ ) and overall efficiency after injection in the device ( $\eta_{\text{det}} \sim 0.1$ )

Higher order emission terms, each occurring with probability proportional to  $g^6$ , corresponding to three photon pairs (two signal pairs and one noise pair), can lead to different input states that cannot be distinguished from the correctly heralded one. Three possible noise combinations may arise. (i) Two pairs are emitted from source  $S_2$  and a pair from source  $S_{\alpha \neq 2}$ , which can lead after loss of two photons to input states of the form  $(2_i, 1_j, 0_k)$ . (ii) One pair is emitted from source  $S_2$  and two pairs from source  $S_{\alpha \neq 2}$ , which can lead after loss of one photon to input states of the form  $(2_i, 1_j, 0_k)$ . (iii) One pair is emitted by each source  $S_2$ ,  $S_{\alpha \neq 2}$  and  $S_{\beta \neq \{\alpha, 2\}}$ , which can lead after loss of one photon to input states of the form  $(1_i, 1_j, 1_l)$ , with  $l$  different from the heralded mode  $k$ . Including all transmission efficiencies and the relative emission probabilities, and using the experimental values for parameters  $g \sim 0.1$ ,  $\eta_D \sim 0.015$  and  $\eta_T \sim 0.2$  the following relative probabilities of different types of events:  $P_{\text{corr}} \sim 0.86$  for correctly heralded inputs,  $P_{\text{noise}, 210} \sim 0.07$  for  $(2_i, 1_j, 0_k)$  noise terms and  $P_{\text{noise}, 111} \sim 0.07$  for  $(1_i, 1_j, 1_l)$  noise terms. Note that  $P_{\text{noise}, 210}$  is a contribution also present in the Standard Boson Sampling protocol and can be reduced by decreasing the gain of each SPDC source.

Our goal now is to estimate the impact of the 14% of incorrectly heralded events in our validation tests. If this fraction of wrongly heralded events behave as white noise, their only effect will be to increase the number of events required for a given confidence level in the validation. We now describe an analysis that shows that these wrongly heralded events are approximately unbiased, and hence have an effect close to that of white noise, for the validation test to discriminate Boson Sampling with indistinguishable and distinguishable photons.

Let us consider an incorrectly heralded input of form  $(1_i, 1_j, 1_l)$ , when the heralded input was  $(1_i, 1_j, 1_k)$ . The validation test will compare events arising from this incorrectly heralded input with two hypotheses:  $A$ , that the event arises from the heralded input  $(1_i, 1_j, 1_k)$ , in a

Boson Sampling experiment with indistinguishable photons; and  $B$ , that the event arises from the heralded input  $(1_i, 1_j, 1_k)$ , but in an experiment with distinguishable photons. We use the total variation distance  $d = \frac{1}{2} \sum_i |p_i - q_i|$  between two probability distributions  $p, q$  to quantify their degree of similarity. We calculate the variation distance  $d(data, A)$  between the output distributions associated with the true input  $(1_i, 1_j, 1_l)$  and the heralded input  $(1_i, 1_j, 1_k)$ . This is to be compared with the variation distance  $d(data, B)$  between the distributions obtained with the true input  $(1_i, 1_j, 1_l)$ , and the distribution obtained with the heralded input, but assuming distinguishable photons. In these calculations, we have included the effect of limited photon indistinguishability. The pair of distances  $(d(data, A), d(data, B))$  is then calculated for all possible pairs of correct/incorrect inputs (there are  $286 \times 285 = 81510$  such pairs). In Fig. 6 a we report a contour plot of the obtained distribution of pairs  $(d(data, A), d(data, B))$ , and observe that the two quantities are strongly correlated. This means that an event sampled from a wrongly heralded input will likely be equally dissimilar to the distributions corresponding to the two hypotheses  $A$  and  $B$  of the validation test. On average, these errors in the input state injection will then merely result in additional white noise in the validation procedure. The same analysis has been carried out for the  $(2_i, 1_j, 0_k)$  contribution (see Fig. 6 b), leading to the same conclusions.

We confirmed this prediction by performing a numerical simulation of a validation test against the distinguishable photon hypothesis, for the specific inputs used in our experiment with the 13-mode chip. The simulation is performed with and without including additional contributions from higher order terms and triggering errors (see Fig.7), and using the parameters of the actual experiment (nonlinear gain of the PDC sources  $g \sim 0.1$ , overall transmissivity  $\eta_D \sim 0.015$ , overall triggering efficiency  $\eta_T \sim 0.20$ ). As expected, we observe that for a fixed sample size, higher order terms result in a lowering of the validation confidence level.

Finally, let us estimate the expected contribution of these errors in future experiments. The triggering error terms are expected to become more relevant for a large number of modes and sources. Fortunately, this problem can be overcome by having each heralding detector quickly open an optical shutter in the corresponding input mode, thus ruling out the possibility of injecting photons into unheralded input modes. This scheme would require an appropriate optical delay line. In the case of a full Scattershot experiment with  $m$  modes and  $m$  sources, the per-pulse probability of detecting an  $n$ -fold coincidence at the output of the chip together with an

$n$ -fold triggering event is:

$$P_{det}^{shutters} = \eta_D^n \sum_{s=n}^m g^s (1-g)^{m-s} \binom{m}{s} \eta_T^n (1-\eta_T)^{s-n} \binom{s}{n}, \quad (4)$$

while without shutters all contributions with  $s \geq n$  photons are present:

$$P_{det}^{noshutters} = \sum_{s=n}^m g^s (1-g)^{m-s} \binom{m}{s} \eta_T^n \eta_D^n (1-\eta_T)^{s-n} (1-\eta_D)^{s-n} \binom{s}{n}^2, \quad (5)$$

where  $\eta_T, \eta_D$  are respectively the triggering efficiency and the detection efficiency (including all losses from generation to detection at the chip's output). The ratio  $R$  between the quantities in Eqs. (5) and (4) provides an estimate of the contribution of untriggered SPDC pairs to the total number of events. In Fig. 8 we plot this quantity for a three-photon experiment as a function of  $m$ , highlighting that shutters start to be necessary already for  $m \sim 20$ .

This work was originally published as Supplementary Materials for Bentivegna et al. *Sci. Adv.* 2015; 1:e1400255, <http://advances.sciencemag.org/content/suppl/2015/04/14/1.3.e1400255.DC1>. The full legal code of the Creative Commons Attribution-NonCommercial 4.0 International Public License may be found at <http://creativecommons.org/licenses/by-nc/4.0/legalcode>.

## References

1. C. Hong, Z. Ou, and L. Mandel. Measurement of subpicosecond time intervals between two photons by interference. *Phys. Rev. Lett.*, 59:2044–2046, 1987.
2. F. De Martini and F. Sciarrino. Non-linear parametric processes in quantum information. *Progress in Quantum Electronics*, 29(3-5):165 – 256, 2005.
3. M. A. Broome, A. Fedrizzi, S. Rahimi-Keshari, J. Dove, S. Aaronson, T. C. Ralph, and A. G. White. Photonic boson sampling in a tunable circuit. *Science*, 339:794–798, 2013.

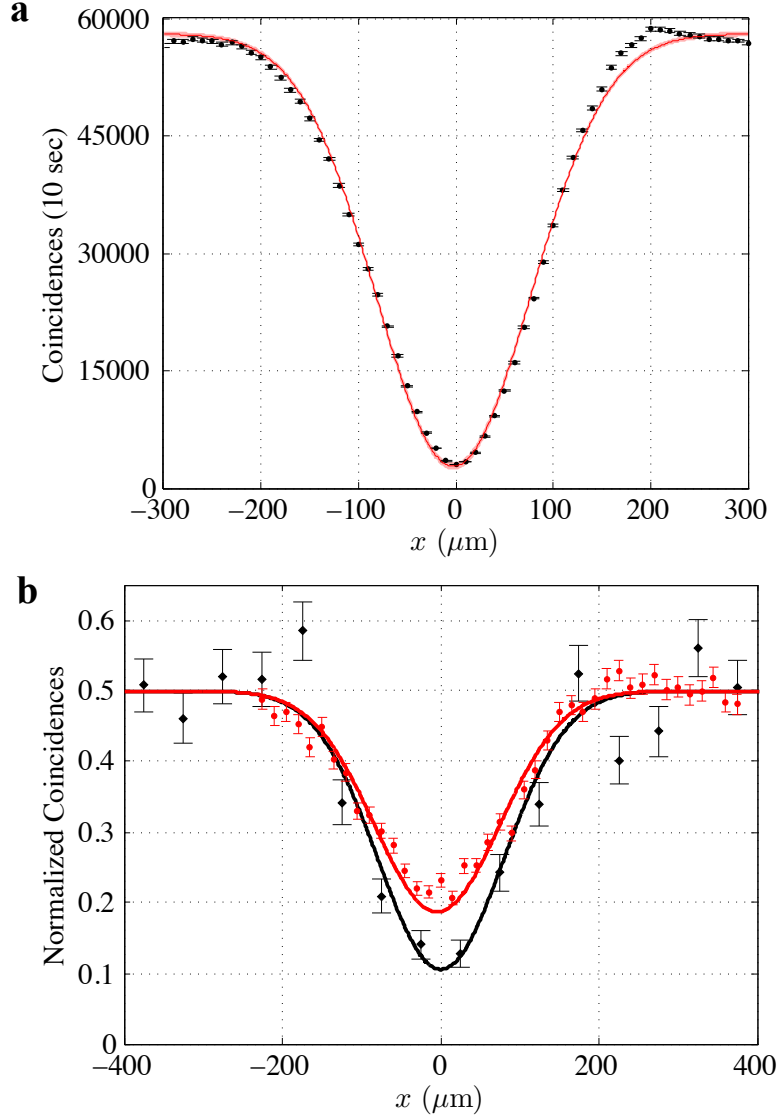

Fig. 1: Characterization of the sources photon indistinguishability by Hong-Ou-Mandel interference in a symmetric beam-splitter. The number of coincidences at two specific outputs for a fixed time-interval is plotted as a function of the spatial delay between the two photons. **a**, Hong-Ou-Mandel interference between photons belonging to the same pair, emitted from source  $S_2$  (crystal  $C_\alpha$ ). The observed visibility is  $V = 0.952 \pm 0.006$ . **b**, Hong-Ou-Mandel interference between photons belonging to different pairs. Black points: Hong-Ou-Mandel interference between photons emitted from sources  $S_1$  and  $S_2$  of the same crystal  $C_\alpha$ , with visibility  $V = 0.63 \pm 0.03$ . Red points: Hong-Ou-Mandel interference between photons emitted from crystals  $C_\alpha$  and  $C_\beta$ , with visibility  $V = 0.79 \pm 0.06$ . Lines: best-fit curves. Coincidences are normalized to the same value at the delay value  $400 \mu\text{m}$ . Error bars are due to the poissonian statistics of the recorder events.

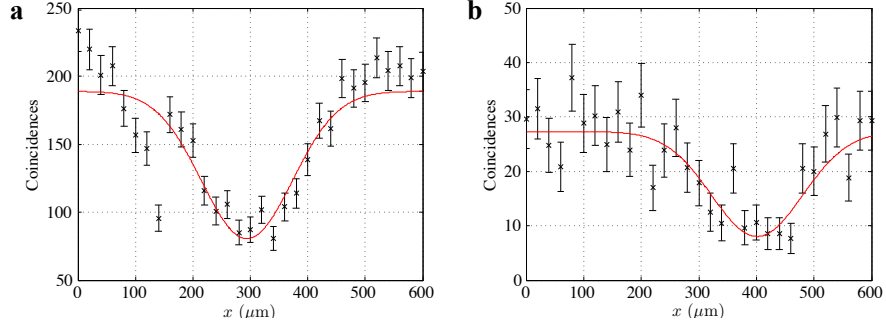

Fig. 2: Synchronization of single photons belonging to the same source obtained by PDC. The number of coincidences at two specific outputs for a fixed time-interval is plotted as a function of the spatial delay between the two photons. The matching position is given by the minimum (maximum) of the dip (peak). **a**, Synchronization between photons injected into modes 6 and 7 (photons generated by the first crystal  $C_\alpha$ ). **b**, Synchronization between photons injected into modes 5 and 9 (photons generated by the second crystal  $C_\beta$ ).

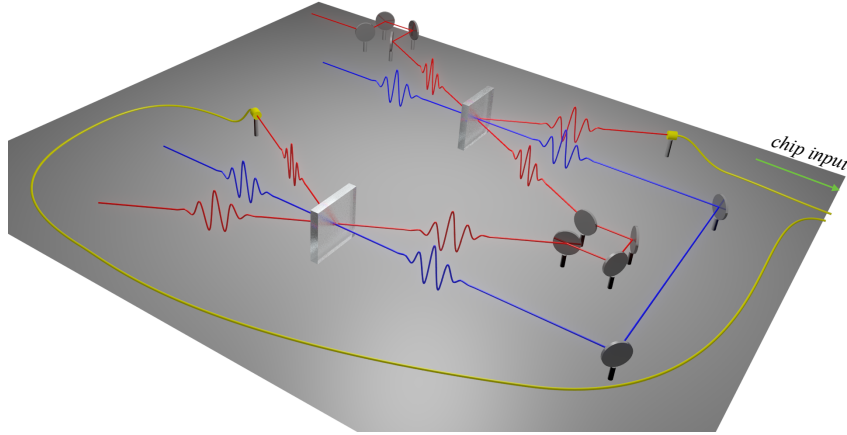

Fig. 3: Scheme to exploit stimulated emission for the synchronization of photons generated from different crystals. The same coherent state is temporally matched with the pump beam in two different crystals. The idler beams generated by the amplification processes are then injected into the chip inputs. The observation of Hong-Ou-Mandel interference between the stimulated fields ensures temporal synchronization of the crystals.

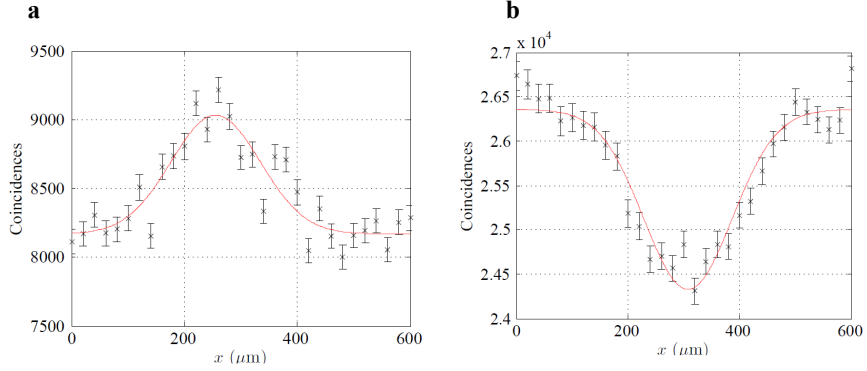

Fig. 4: Synchronization of single photons belonging to different sources obtained by amplification of coherent states. The number of coincidences at two specific outputs for a fixed time-interval is plotted as a function of the spatial delay between the two beams. The matching position is given by the minimum (maximum) of the dip (peak). **a**, Synchronization between photons injected into modes 6 (photon generated by the first crystal) and 9 (photon generated by the second crystal). **b**, Synchronization between photons injected into modes 6 (photon generated by the first crystal) and 12 (photon generated by the third crystal). Points: experimental data. Lines: best-fit curves. Error bars are due to the poissonian statistics of the recorded events. The time interval for each of the experimental data is 60s.

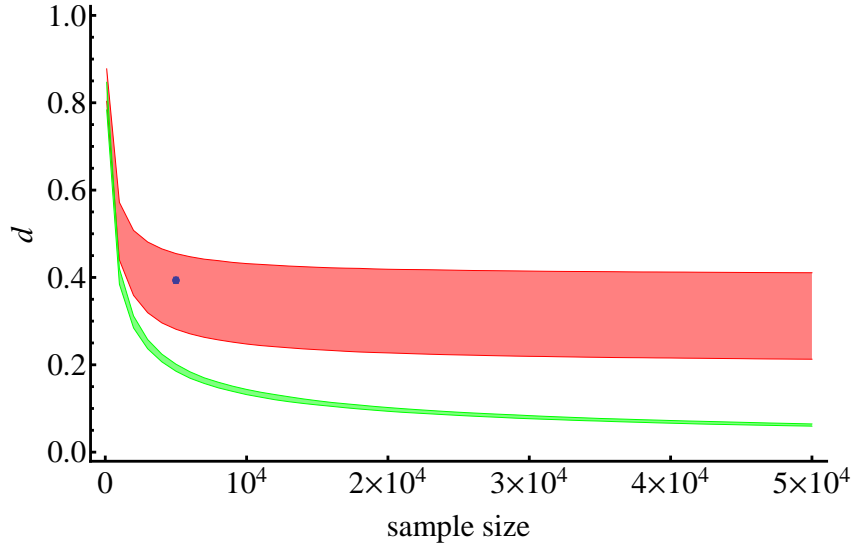

Fig. 5: Dependence of the variation distance  $d$  as a function of the sample size. Red region:  $2\sigma$  region from a numerical simulation including errors on the unitary, averaged over 100 random unitaries within fabrication tolerances. Green region:  $2\sigma$  region from a numerical simulation with the ideal, theoretical unitary. Blue point: experimental value of the variation distance  $d$  for the 13-mode Scattershot experiment.

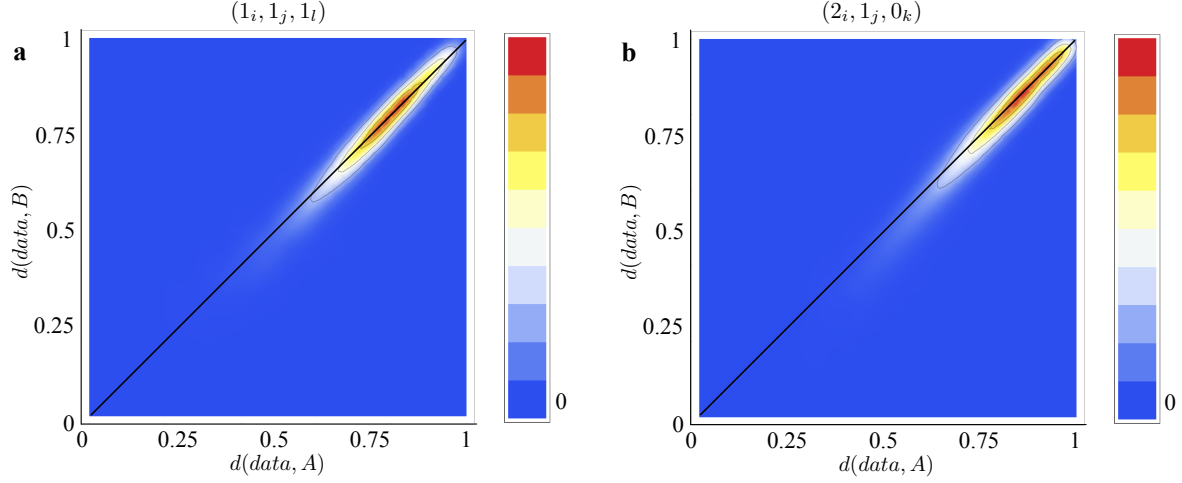

Fig. 6: Contour plot of distribution of pairs  $(d(\text{data}, A), d(\text{data}, B))$  of variation distances between the output distribution associated with an incorrectly heralded event, and either the hypothesis of correct heralded input ( $A$ ), or the hypothesis of correct input but using distinguishable photons ( $B$ ). Left plot: distribution of events corresponding to  $(1_i, 1_j, 1_l)$  incorrect states; right plot: distribution of events corresponding to  $(2_i, 1_j, 0_k)$  incorrect states. The high values obtained for both variation distances indicate incorrect heralds result in output distributions which are significantly different from the expected ones, whereas strong correlation between the two members of the pair indicate unbiasedness between the two hypotheses.

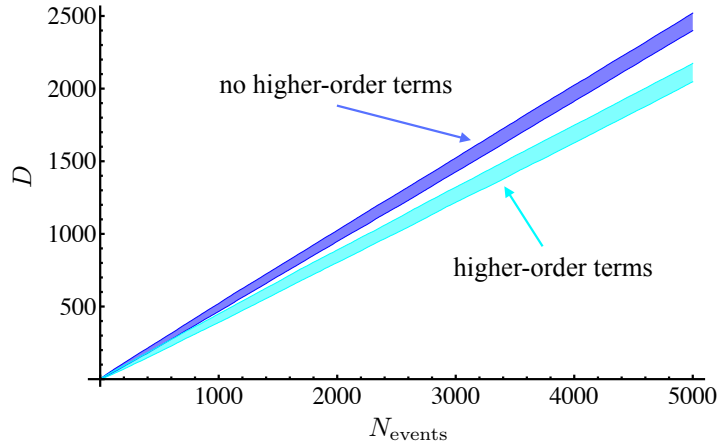

Fig. 7: Numerical simulation of a validation test of simulated experimental data against the hypotheses of correct Boson Sampling data ( $D > 0$ ), and the hypothesis that photons are distinguishable ( $D < 0$ ). The test results are averages over 100 different realizations, with (light blue region) and without (dark blue region) additional contribution of higher order terms, in the specific case of our experimental parameters and input state combinations. The shaded regions correspond to  $1\sigma$  confidence intervals.

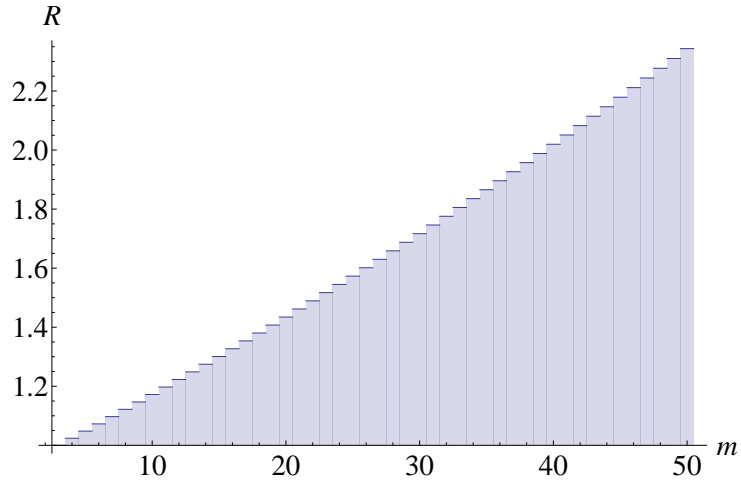

Fig. 8: Ratio  $R = P_{det}^{no\ shutters} / P_{det}^{shutters}$  between the per-pulse probability of detecting 3 photons in the trigger apparatus and 3 photons after the chip without shutters and with shutters, as a function of the number  $m$  of sources and modes ( $g = 0.1$ ,  $\eta_T = 0.2$ ,  $\eta_D = 0.015$ ).
